# Supplementary material for: Rotate Your Character: Revisiting Video Diffusion Models for High-Quality 3D Character Generation
Source: arXiv:2601.05722 source file (2026-01-09)
Supplement: Supplementary file 1 [file X_suppl.tex]

\clearpage
\setcounter{page}{1}
\maketitlesupplementary
